# Supplementary material for: Better Aggregation in Test-Time Augmentation
Source: arXiv:2011.11156 source file (2021-10-11)
Supplement: Supplementary file 1 [file supplement.tex]

\section{Implementation Details}
